# Supplementary material for: Sort-free Gaussian Splatting via Weighted Sum Rendering
Source: arXiv:2410.18931 source file (2025-04-09)
Supplement: Supplementary file 2 [file a_appendix.tex]

%===============================================================================
\subsection{Weighted Sum Updates}
%===============================================================================

Equations \ref{eq:10} and \ref{eq:12} use exponential functions for computing color vector weights because they simplify updating weighted sums in a manner that avoids losing precision with weight numerical underflow. In this section it is shown how the sums can be efficiently computed such that the weights are normalized by the largest weight.

We exploit the fact that the quotient of weighted sums, as in eqs. \ref{eq:10} and \ref{eq:12}, are not affected by adding constants to the exponent. For example, assuming we have two functions such that $\tilde{d}\left(z,\mathbf{w}\right)=d\left(z,\mathbf{w}\right)+\xi$, and use them in a quotient of weighted sums. This results in

\begin{equation}
\frac{\sum_{i=0}^{N}a_{i}e^{-\bar{d}\left(z_{i},\mathbf{w}\right)}}{\sum_{i=0}^{N}b_{i}e^{-\bar{d}\left(z_{i},\mathbf{w}\right)}}=\frac{e^{-\xi}\sum_{i=0}^{N}a_{i}e^{-\bar{d}\left(z_{i},\mathbf{w}\right)}}{e^{-\xi}\sum_{i=0}^{N}b_{i}e^{-\bar{d}\left(z_{i},\mathbf{w}\right)}}=\frac{\sum_{i=0}^{N}a_{i}e^{-d\left(z_{i},\mathbf{w}\right)}}{\sum_{i=0}^{N}b_{i}e^{-d\left(z_{i},\mathbf{w}\right)}}
\label{eq:13}
\end{equation}

i.e., the result is the same.

This property can be used while updating the weighted sums in eqs. \ref{eq:10} and \ref{eq:12}. Defining

\begin{equation}
\mu_{k}=\underset{i=0,1,\cdots,k}{\min}d\left(z_{i},\mathbf{w}\right),k=0,1,\cdots,N
\label{eq:14}
\end{equation}

and

\begin{equation}
\sigma_{k}\left(\mathbf{c}\right)=e^{\mu_{k}}\sum_{i=0}^{k}c_{i}e^{-d\left(z_{i},\mathbf{w}\right)},k=0,1,\cdots,N
\label{eq:15}
\end{equation}

we have

\begin{equation}
\sigma_{k}\left(\mathbf{c}\right)=e^{\mu_{k}-d\left(z_{k},\mathbf{w}\right)}c_{k}+e^{\mu_{k}-\mu_{k-1}}\sigma_{k-1}
\label{eq:16}
\end{equation}

This means that we can update $\mu_{k}$, $\sigma_{k}$ from  $\mu_{k-1}$, $\sigma_{k-1}$ as

\begin{equation}
\mu_{k}=\min\left(d\left(z_{i},\mathbf{w}\right),\mu_{k-1}\right)
\label{eq:17}
\end{equation}

\begin{equation}
\sigma_{k}\left(\mathbf{c}\right)=\begin{cases}
c_{k}+e^{d\left(z_{k},\mathbf{w}\right)-\mu_{k-1}}\left(\mathbf{c}\right) & d\left(z_{k},\mathbf{w}\right)<\mu_{k-1}\\
e^{\mu_{k-1}-d\left(z_{k},\mathbf{w}\right)}c_{k}+\sigma_{k-1}\left(\mathbf{c}\right) & \text{\text{otherwise}}
\end{cases}
\label{eq:18}
\end{equation}

and obtain the final desired result from the quotient of sums with normalized weights

\begin{equation}
\frac{\sum_{i=0}^{N}a_{i}e^{-d\left(z_{i},\mathbf{w}\right)}}{\sum_{i=0}^{N}b_{i}e^{-d\left(z_{i},\mathbf{w}\right)}}=\frac{e^{-\mu_{N}}\sum_{i=0}^{N}a_{i}e^{-d\left(z_{i},\mathbf{w}\right)}}{e^{-\mu_{N}}\sum_{i=0}^{N}b_{i}e^{-d\left(z_{i},\mathbf{w}\right)}}=\frac{\sigma_{N}\left(\mathbf{a}\right)}{\sigma_{N}\left(\mathbf{b}\right)}
\label{eq:19}
\end{equation}

%===============================================================================
\subsection{Two-pass gradient computation}
%===============================================================================

Similarly to other machine learning problem, the GS-WSR parameters are determined by minimizing a loss function over a training set. In this case this set is defined by a set of views as shown in Figure 2. Using $\mathbf{R}_v$ and $\mathbf{S}_v$ to represent respectively the rendered views and the training set images, with pixel values $\mathbf{r}_{v}\left[m,n\right]$ and $\mathbf{s}_{v}\left[m,n\right]$, the average loss for a given error function $D$ is
\begin{equation}
L=\frac{1}{VHW}\sum_{v=1}^{V}\sum_{m=1}^{H}\sum_{n=1}^{W}D\left(\mathbf{r}_{v}\left[m,n\right],\mathbf{s}_{v}\left[m,n\right]\right)
\label{eq:21}
\end{equation}

During optimization it is necessary to compute partial derivatives of $L$ with respect to all model parameters. Using $\mathcal{P}_i$ to represent the set with all parameters of the GS element with index $i$, it is necessary to compute
\begin{equation}
\frac{\partial L}{\partial\tau_{i}},\text{for all }\tau\in\mathcal{P}_{i}
\label{eq:22}
\end{equation}

To simplify notation, we assume that the loss function in eq. \ref{eq:21} is fully separable per pixel, and drop the image and pixel indexes to represent a pixel color vector $\mathbf{r}$, and also replace $d\left(z_i,\mathbf{w}\right)$ with $d_i$ to define a single pixel color vector as
\begin{equation}
\mathbf{r}=\frac{\sum_{i=0}^{N}\mathbf{c}_{i}\alpha_{i}e^{-d_{i}}}{\sum_{i=0}^{N}\alpha_{i}e^{-d_{i}}}
\label{eq:23}
\end{equation}
where it is implicitly assumed that $\mathbf{c}_i$, $\alpha_i$, $d_i$ may depend on a parameter represented simply as $\tau_i$.

With this notation, it is necessary to compute the partial derivatives
\begin{equation}
\frac{\partial D\left(\mathbf{r},\mathbf{s}\right)}{\partial\tau_{i}}=\sum_{l=1}^{3}\frac{dD\left(r_{l},s_{l}\right)}{dr_{l}}\frac{\partial r_{l}}{\partial\tau_{i}},\text{for all \ensuremath{\tau_{i}\in}\ensuremath{\mathcal{P}_{i}}}
\label{eq:24}
\end{equation}
where
\begin{equation}
r_{l}=\frac{\sum_{i=0}^{N}c_{i,l}\alpha_{i}e^{-d_{i}}}{\sum_{i=0}^{N}\alpha_{i}e^{-d_{i}}}
\label{eq:25}
\end{equation}

This corresponds to
\begin{equation}
\frac{\partial D\left(\mathbf{r},\mathbf{s}\right)}{\partial\tau_{i}}=\frac{1}{\sum_{i=0}^{N}\alpha_{i}e^{-d_{i}}}\sum_{l=1}^{3}\frac{dD\left(r_{l},s_{l}\right)}{dr_{l}}\left[\left(\alpha_{i}e^{-d_{i}}\right)\frac{\partial c_{i,l}}{\partial\tau_{i}}+\left(c_{i,l}-r\right)\left(\frac{\partial\left(\alpha_{i}e^{-d_{i}}\right)}{\partial\tau_{i}}\right)\right]
\label{eq:26}
\end{equation}

Since eq.~\ref{eq:23} is a fraction of two summations, the parameter partial derivatives depend on the final summation values. Those per-pixel values can be computed with a single rendering pass, and in a second pass, the full gradient can be computed using eq.~\ref{eq:26}.

The important observation is that GS-WSR can also be more efficient during the optimization stage because no sorting is needed in either gradient determination pass, and thus all the computations can all be done independently for each GS-WSR element (i.e., in parallel).

%===============================================================================
\subsection{Simplified color representation}
%===============================================================================

The original 3DGS method uses up to 16 spherical harmonics parameters per 3-dimensional color vector component, with a total of 48 parameters. The addition of view-dependent opacity helps improve results obtained with GS-WSR, but at the cost of adding 16 more spherical harmonics parameters to each element, totaling 64 parameters.

To reduce the number of parameters we can exploit the fact that the most common form of view-dependent color variations is defined by specular reflections, which can be approximated with a single color, but with varying intensity.

This can be obtained with a scalar function $x\left(\mathbf{f}-\mathbf{p},\mathbf{h}\right)$ that depends on view direction and spherical harmonics parameters (up to 16 if using the same set as 3DGS), and in eq.~(\ref{eq:9}) use the following definition for the color vector

\begin{equation}
\mathbf{c}\left(\mathbf{f}-\mathbf{p},\mathbf{h}\right)=a+x\left(\mathbf{f}-\mathbf{p},\mathbf{h}\right)\mathbf{b}
\label{eq:20}
\end{equation}

where $\mathbf{a}$, $\mathbf{b}$, and $\mathbf{h}$ are learned parameters.

\subsection{GS-WSR full presentation}

Machine learning is the fundamental technique that enables high-quality new view synthesis, since they provide powerful ways to create good data representations using only training data.

In this sense, 3DGS is one specific type of representation and rendering, which is optimized using machine learning. Thus, it can be modified to a representation that is computationally more efficient, and the machine learning techniques adjusted to optimize the parameters of the new representation.

The first generalization is to modify equations \ref{eq:3DGSalpha} and \ref{eq:3DGScolor}, which define the Gaussian Splatting elements shape, color, and opacity, replacing the 3DGS element’s maximum opacity $t_{i}\in\left[0,1\right]$ with an unconstrained value $u_{i}\left(\mathbf{f}-\mathbf{p}_{i},\mathbf{t}_{i}\right)$, that depends on view direction according to learned spherical harmonics parameter vector $\mathbf{t}_{i}$. 

The new equations defining shape, color, and opacity of each GS element are

\begin{equation}
\alpha_{i}\left(\mathbf{x}_{i},\mathbf{t}_{i}\right)=u_{i}\left(\mathbf{f}-\mathbf{p}_{i},\mathbf{t}_{i}\right)\exp\left(-\frac{\left(\mathbf{x}-\mathbf{p}_{i}\right)^{t}\left[\sum\left(\mathbf{q}_{i},\mathbf{s}_{i}\right)\right]^{-1}\left(\mathbf{x}-\mathbf{p}_{i}\right)}{2}\right)
\label{eq:8}
\end{equation}

and

\begin{equation}
\mathbf{r}_{i}\left(\mathbf{x},\mathbf{f}\right)=\alpha_{i}\left(\mathbf{x}_{i},\mathbf{t}_{i}\right)\mathbf{c}\left(\mathbf{f}-\mathbf{p}_{i},\mathbf{h}_{i}\right),i=1,2,\cdots,N
\label{eq:9}
\end{equation}

With this new formulation for color and opacity, after employing the same discretization used for the original 3DGS method, pixel values can be computed according to

\begin{equation}
\mathbf{r}\left[m,n\right]=\bar{\alpha}\left[m,n\right]\mathbf{c}_{0}\left[m,n\right]+\left(1-\bar{\alpha}\left[m,n\right]\right)\frac{\sum_{i=1}^{=N}\mathbf{c}_{i}\left[m,n\right]\alpha_{i}\left[m,n\right]e^{-d\left(z_{i},\mathbf{w}\right)}}{\sum_{i=1}^{=N}\alpha_{i}\left[m,n\right]e^{-d\left(z_{i},\mathbf{w}\right)}}
\label{eq:10}
\end{equation}

where $\mathbf{c}_{0}\left[m,n\right]$ is the background color, $d\left(z_{i},\mathbf{w}\right)$ is a positive function that depends on element’s depth $z_i$ and a vector of learned parameters $\mathbf{w}$. For instance, we can use the following function with two learned parameters 

\begin{equation}
d\left(z_{i},\mathbf{w}\right)=w_{o}\left|z_{i}\right|w^{1}
\label{eq:11}
\end{equation}

Note that rendering with eq. \ref{eq:10} corresponds to only computing weighted sums, visiting the new GS elements in any order. For that reason, it is called Gaussian Splatting with weighted sum rendering (GS-WSR).

This GS-WSR formulation is similar to OIT eq. \ref{eq:6} and requires computing values of $\bar{\alpha}_{i}\in\left[m,n\right]$ for each pixel. This requirement can be eliminated by using a simplified version of GS-WSR, where a depth for scene background is learned and pixels values are computed using 

\begin{equation}
\mathbf{r}\left[m,n\right]=\frac{\sum_{i=1}^{=N}\mathbf{c}_{i}\left[m,n\right]\alpha_{i}\left[m,n\right]e^{-d\left(z_{i},\mathbf{w}\right)}}{\sum_{i=1}^{=N}\alpha_{i}\left[m,n\right]e^{-d\left(z_{i},\mathbf{w}\right)}}
\label{eq:12}
\end{equation}

where $\alpha_{0}\left[m,n\right]=1$, and $z_0$ is the learned background depth.

While 3DGS can be considered a conventional graphics technique that is augmented with machine learning tools, this formulation departs from physics-based assumptions, and instead relies more on the machine learning to work.

For instance, alpha blending is based on the physical principles of light transmittance and absorption. Thus, in eq. \ref{eq:5} it is necessary to have $\alpha_{i}\in\left[0,1\right]$ to guarantee that all terms are positive. However, those requirements are not required for eqs. \ref{eq:10} and \ref{eq:12} because, in the machine learning framework, $\alpha_{i}$ are simply parameters in a radiance field model, and thus removing constraints can potentially result in better approximations.

Similarly, the view-dependent opacity $u_{i}\left(\mathbf{f}-\mathbf{p}_{i},\mathbf{t}_{i}\right)$ used in eq. \ref{eq:8} may not correspond to optical laws, but it is in practice useful for minimizing the limitations of rendering eq. \ref{eq:6} compared to blending eq. \ref{eq:5}.

\subsection{More results}

We show more visual comparison in Figure~\ref{fig:nerfsyn1} and Figure~\ref{fig:nerfsyn2} on the Synthetic NeRF dataset. We also show more results in Figure~\ref{fig:mipnerf1} and Figure~\ref{fig:mipnerf2}.

\begin{figure*}
\centering
  \includegraphics[width=1.0\textwidth]{iclr2025/Figs/nerfsyn_1.png}\vspace{-0.15in}
  \caption{
    More visual comparison on the Synthetic NeRF dataset.
  }\vspace{-0.2in} 
  \label{fig:nerfsyn1} 
\end{figure*}

\begin{figure*}
\centering
  \includegraphics[width=1.0\textwidth]{iclr2025/Figs/nerfsyn_2.png}\vspace{-0.15in}
  \caption{
    More visual comparison on the Synthetic NeRF dataset.
  }\vspace{-0.2in} 
  \label{fig:nerfsyn2} 
\end{figure*}

\begin{figure*}
\centering
  \includegraphics[width=1.0\textwidth]{iclr2025/Figs/mipnerf_1.png}\vspace{-0.15in}
  \caption{
    More visual comparison on the Mip-NeRF360 dataset, the Tanks\&Temples dataset, and the Deep Blending dataset.
  }\vspace{-0.2in} 
  \label{fig:mipnerf1} 
\end{figure*}

\begin{figure*}
\centering
  \includegraphics[width=1.0\textwidth]{iclr2025/Figs/mipnerf_2.png}\vspace{-0.15in}
  \caption{
    More visual comparison on the Mip-NeRF360 dataset, the Tanks\&Temples dataset, and the Deep Blending dataset.
  }\vspace{-0.2in} 
  \label{fig:mipnerf2} 
\end{figure*}

% Help me revise the following text from an academic paper, make it academic, grammatically correct, stronger, and more convincing:

% Fix spelling and grammar. Make sentences more clear and concise. Split up run-on sentences. Reduce repetition. When replacing words, do not make them more complex or difficult than the original. If the text contains quotes, repeat the text inside the quotes verbatim. Keep the original markdown format. Do not use overly formal language.
% Input:
